# Supplementary material for: MCTS Based Dispatch of Autonomous Vehicles under Operational Constraints for Continuous Transportation
Source: arXiv:2407.16200 source file (2024-07-23)
Supplement: Supplementary file 1 [file appendix.tex]

\appendix

\section{Additional Figures}
Figures to show tuning results of capacity, ratio constraints and window constraints, and comparison of proposed work against \fasthc -- FAST with heurisitic controllers. 

\begin{figure*}[t]
	\centering
	\includegraphics[width=1.9\columnwidth]{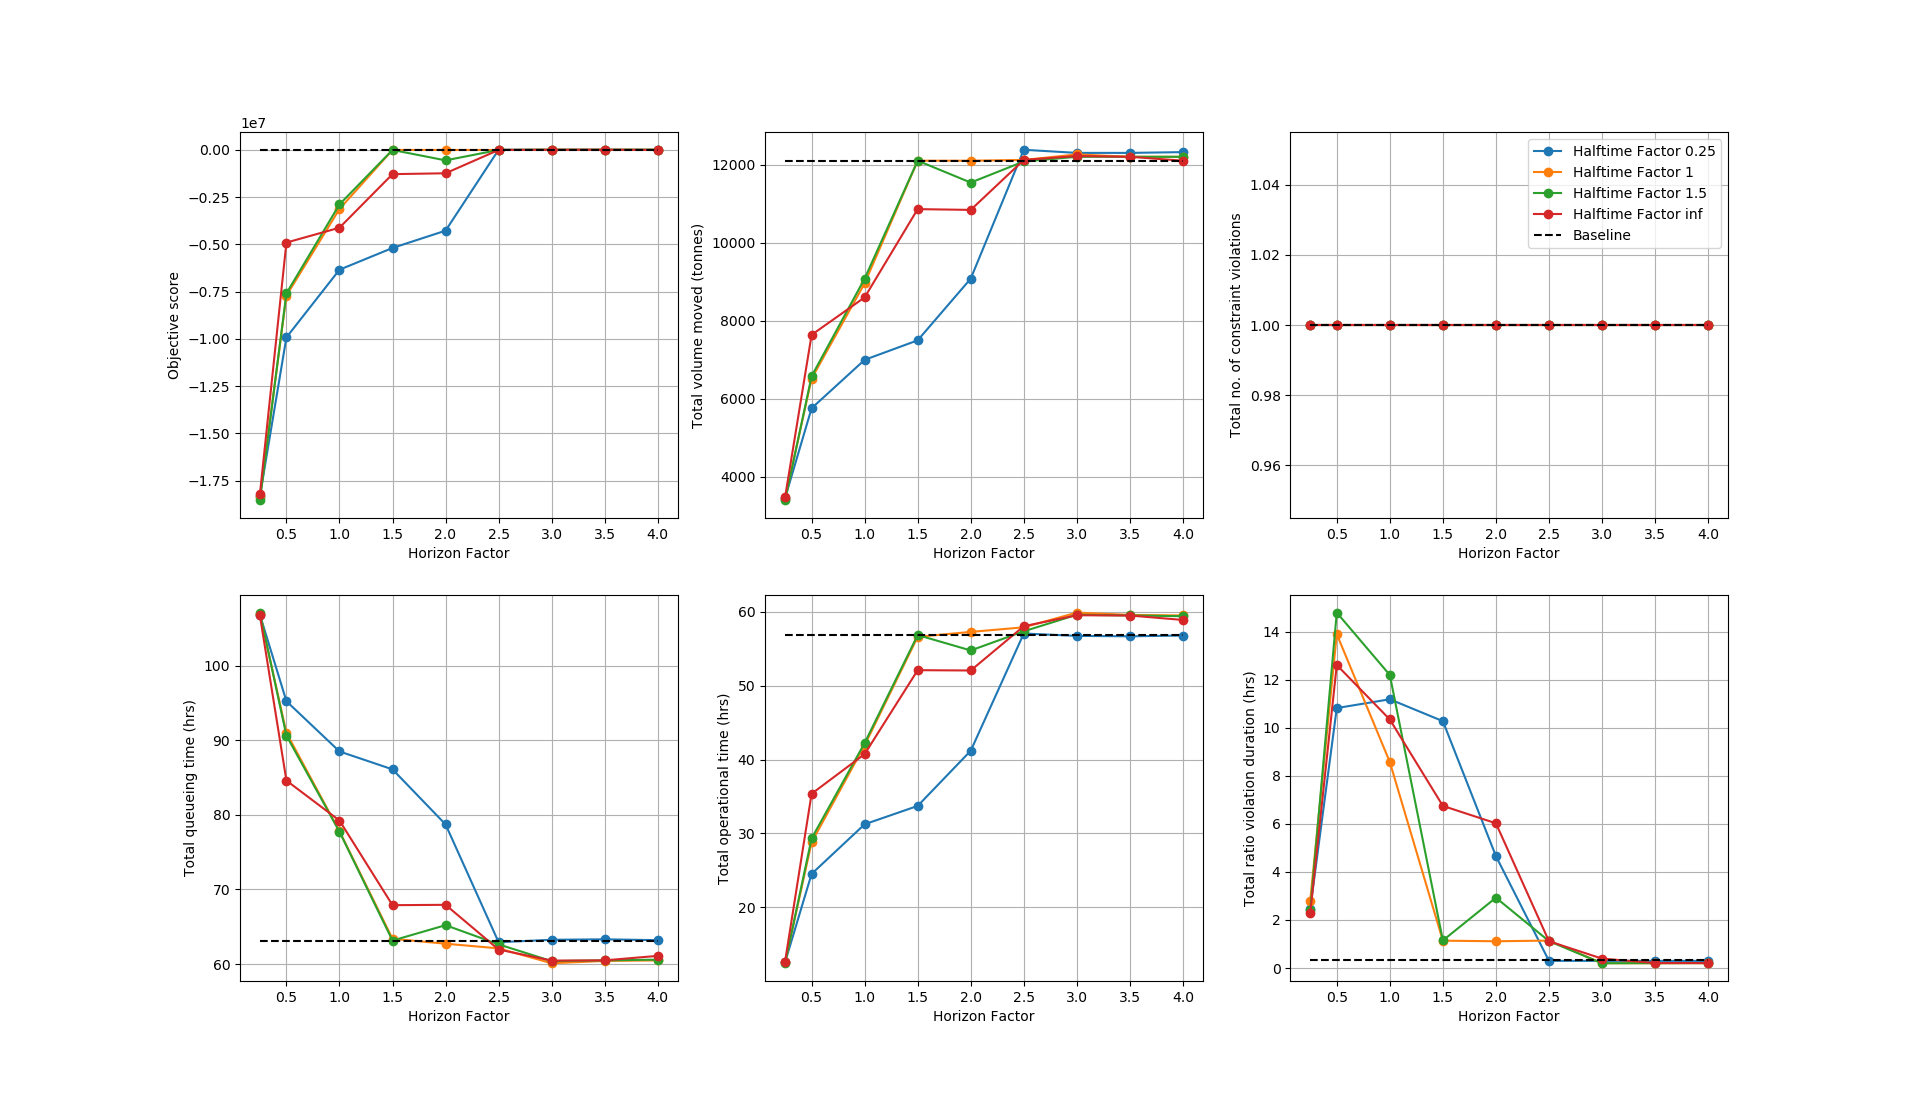}
	\caption{Performance indicators for varying horizon and constant discounting values for FAST with capacity and ratio constraints}
	\label{kpicapacityratio}
\end{figure*}

\begin{figure*}[t]
	\centering
	\includegraphics[width=1.9\columnwidth]{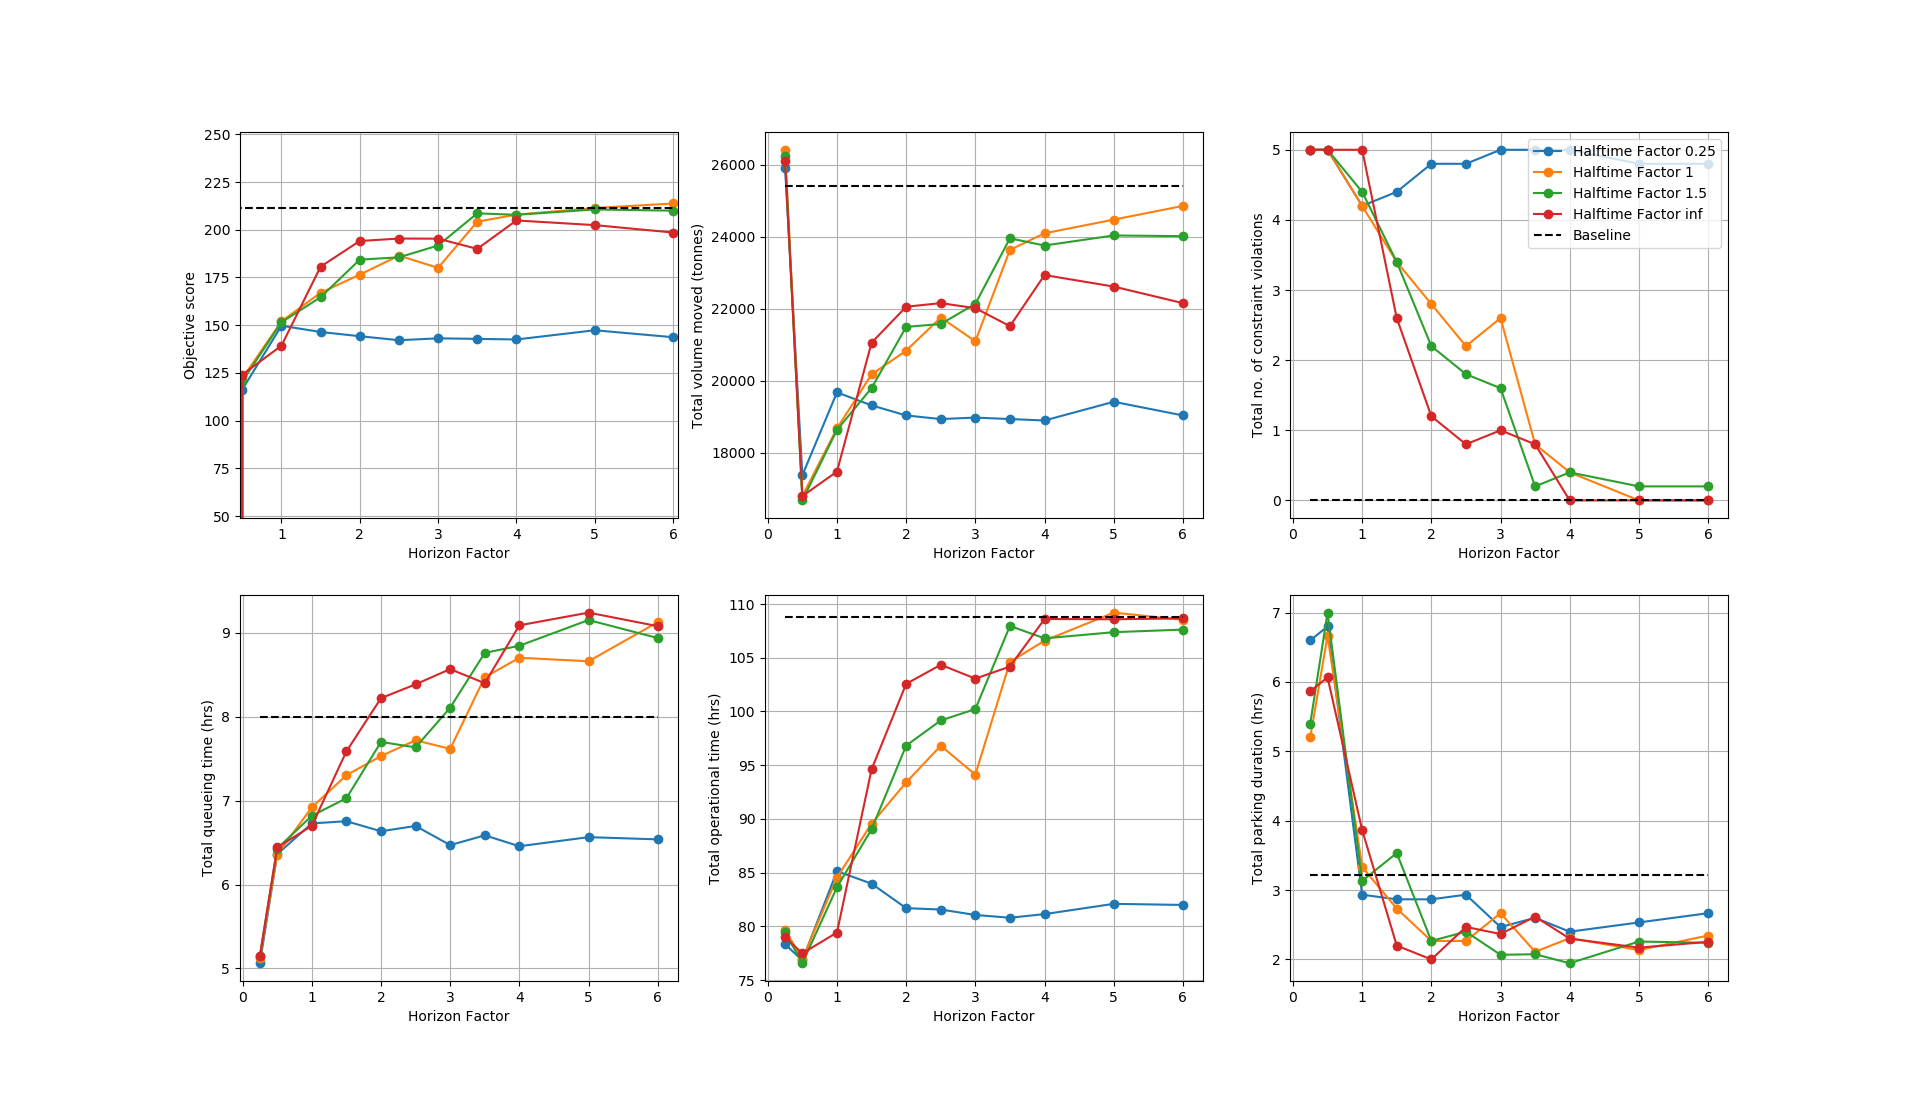}
	\caption{Performance indicators for varying horizon and constant discounting values for FAST with window constraints}
	\label{kpiwindow}
\end{figure*}
